# Supplementary material for: The Integrated Probabilistic Data Association Filter Adapted to Lie Groups
Source: arXiv:2108.07265 source file (2022-10-14)
Supplement: Supplementary file 5 [file A1_LemmaPredictionStep_diff.tex]

\section{Proof of Lemma~\ref{lem:lgipdaf_belief_measurement}: Prediction Step}
\label{app:lgipdaf_proof_prediction}
\begin{proof}
According to the theorem of total probability, the probability of the track's current state conditioned on the previous measurements and \DIFdelbegin \DIFdel{it }\DIFdelend \DIFaddbegin \DIFadd{the track }\DIFaddend representing the target is
\DIFdelbegin %DIFDELCMD < 

%DIFDELCMD < %%%
\DIFdelend \begin{align}\label{eq:lgipdaf_belief_pdf}
p\left(x_{k} \mid \epsilon_{k^-}, Z_{0:k^-} \right)  &=\int_{\tilde{x}_{k^{-} \mid k^{-}}}  p\left(x_{k }\mid x_{k^{-}}, \epsilon_{k^-} , Z_{0:k^-} \right) \notag\\
&p\left(x_{k^{-}} \mid \epsilon_{k^-}, Z_{0:k^-} \right)d \tilde{x}_{k^{-} \mid k^{-}}, \end{align}
where we integrate over the error state instead of the state by recalling that $\tilde{x}_{k^- \mid k^-}= \LogI{\G{x}}{ \hat{x}_{k^- \mid k^-}^{-1} x_{k^-} }$, and using the relation in equation~\eqref{eq:prob_x_def}.

\DIFdelbegin \DIFdel{Substituting in }\DIFdelend \DIFaddbegin \DIFadd{Using }\DIFaddend the definitions of $p\left(x_{k }\mid x_{k^{-}}, \epsilon_{k^-} , Z_{0:k^-} \right)$ and $p\left(x_{k^{-}} \mid \epsilon_{k^-}, Z_{0:k^-} \right)$ \DIFdelbegin \DIFdel{stated in equations}\DIFdelend \DIFaddbegin \DIFadd{in Equations}\DIFaddend ~\eqref{eq:lgipdaf_state_previous} and\DIFaddbegin \DIFadd{~}\DIFaddend \eqref{eq:lgipdaf_approx_state_propagation}\DIFdelbegin \DIFdel{into equation}\DIFdelend \DIFaddbegin \DIFadd{, Equation}\DIFaddend ~\eqref{eq:lgipdaf_belief_pdf} \DIFdelbegin \DIFdel{and combining the exponents yields
}%DIFDELCMD < 

%DIFDELCMD < %%%
\DIFdelend \DIFaddbegin \DIFadd{becomes 
}\DIFaddend \begin{equation}\label{eq:lgipdaf_prob_with_L}
p\left(x_{k} \mid \epsilon_{k^-}, Z_{0:k^-} \right)\approx\eta\int_{\tilde{x}_{k^{-} \mid  k^{-}}}\exp\left(-L\right)d \tilde{x}_{k^{-} \mid  k^{-}},    
\end{equation}
where
\begin{align*}
L&=\frac{1}{2}\left(\tilde{x}_{k\mid k^{-}}-F_{\kt}\tilde{x}_{k^{-} \mid  k^{-}}\right)^{\top}\bar{Q}_{\kt}^{-1}\left(\tilde{x}_{k\mid k^{-}}-F_{\kt}\tilde{x}_{k^{-} \mid  k^{-}}\right)\\
&+\frac{1}{2}\tilde{x}_{k^{-} \mid  k^{-}}^{\top}P_{k^{-} \mid  k^{-}}^{-1}\tilde{x}_{k^{-} \mid  k^{-}},    
\end{align*}
and \DIFaddbegin \DIFadd{where }\DIFaddend $\bar{Q}_{\kt}$ is defined in equation~\eqref{eq:lgipdaf_q_bar}.  \DIFdelbegin \DIFdel{Using }\DIFdelend \DIFaddbegin \DIFadd{After some }\DIFaddend algebra we get
\begin{multline*}
    L= \frac{1}{2} \Big\{
    \xtkmkm^\top (\Pkmkm^{-1} + F_\kt^\top \bar{Q}_\kt^{-1}F_\kt) \xtkmkm
    \\
    + \xtkkm^\top \bar{Q}_{\kt}^{-1} \xtkkm 
    - \xtkkm \bar{Q}_\kt^{-1}F_\kt\xtkmkm 
    \\
    - \xtkmkm^\top F_\kt^\top \bar{Q}_\kt^{-1} \xtkkm
    \Big\} 
\end{multline*}
Defining \DIFdelbegin \DIFdel{$S\stackrel{\triangle}{=} \Pkmkm^{-1} + F_\kt^\top \bar{Q}_\kt^{-1}F_\kt$ }\DIFdelend \DIFaddbegin \DIFadd{$S \defeq \Pkmkm^{-1} + F_\kt^\top \bar{Q}_\kt^{-1}F_\kt$ }\DIFaddend gives
\begin{multline*}
    L= \frac{1}{2} 
    (\xtkmkm-S^{-1}F_\kt^\top\bar{Q}_\kt^{-1}\xtkkm)^\top 
    \\
    S (\xtkmkm-S^{-1}F_\kt^\top\bar{Q}_\kt^{-1}\xtkkm)
    \\
    + \frac{1}{2}\xtkkm\big(\bar{Q}_\kt^{-1} - \bar{Q}_\kt^{-1} F_\kt S^{-1} F_\kt^\top \bar{Q}_\kt^{-1}\big)\xtkkm.
\end{multline*}
Using the matrix inversion lemma
\begin{multline*}
    \bar{Q}_\kt^{-1} - \bar{Q}_\kt^{-1} F_\kt (F_\kt^\top \bar{Q}_\kt^{-1} F_\kt + \Pkmkm^{-1})^{-1}F_\kt^\top \bar{Q}_\kt^{-1} 
    \\
    = (F_\kt \Pkmkm F_\kt^\top + \bar{Q}_\kt)^{-1}
\end{multline*}
gives
\begin{multline*}
    L= L_1(\xtkmkm, \xtkkm)
    \\
    + \frac{1}{2}\xtkkm(F_\kt \Pkmkm F_\kt^\top + \bar{Q}_\kt)^{-1}\xtkkm\DIFdelbegin \DIFdel{.
}\DIFdelend \DIFaddbegin \DIFadd{,
}\DIFaddend \end{multline*}
% Substituting into Equaton~\eqref{eq:lgipdaf_prob_with_L} and noting that $\exp(-L_1(\xtkmkm, \xtkkm)$ is a Gaussian random variable in $\xtkmkm$ (with mean depending on $\xtkkm$) that integrates to a constant that is independent of $\xtkkm$, we get that 
\DIFdelbegin %DIFDELCMD < 

%DIFDELCMD < %%%
\DIFdelend %DIF >  
%DIF >  
%DIF >  
% Taking the first and second derivatives of $L$ w.r.t. $\tilde{x}_{k^{-} \mid  k^{-}}$ yields
% \begin{subequations}\label{eq:lgipdaf_L_partial_derivatives}
% \begin{align}
% \frac{\partial L}{\partial\tilde{x}_{k^{-} \mid  k^{-}}} & =-\left(\tilde{x}_{k\mid k^{-}}-F_{\kt}\tilde{x}_{k^{-} \mid  k^{-}}\right)^{\top}\bar{Q}_{\kt}F_{\kt} \notag \\
% &+\tilde{x}_{k^{-} \mid  k^{-}}^{\top}P_{k^{-} \mid  k^{-}}^{-1} \\
% \frac{\partial^{2}L}{\partial\tilde{x}_{k^{-} \mid  k^{-}}^{2}} & = \Psi^{-1}\triangleq F_{\kt}^{\top}\bar{Q}_{\kt}F_{\kt}+P_{k^{-} \mid  k^{-}}^{-1}.
% \end{align}
% \end{subequations}
% Setting the first derivative to zero and solving for $\tilde{x}_{k^{-} \mid  k^{-}}$
% yields
% \[
% \tilde{x}_{k^{-} \mid  k^{-}}=\Psi F_{\kt}^{\top}\bar{Q}_{\kt}^{-1}\tilde{x}_{k}.
% \]
\DIFdelbegin %DIFDELCMD < 

%DIFDELCMD < %%%
\DIFdelend %DIF > 
% Using the first and second partial derivatives of $L$ in equation~\eqref{eq:lgipdaf_L_partial_derivatives} we construct the term
% \begin{align*}
% L_1\left(\tilde{x}_{k\mid k^{-}},\tilde{x}_{k^{-} \mid  k^{-}}\right) & =\frac{1}{2}\left(\tilde{x}_{k^{-} \mid  k^{-}}-\Psi F_{\kt}^{\top}\bar{Q}_{\kt}^{-1}\tilde{x}_{k\mid k^{-}}\right)^{\top}\\
%  & \Psi^{-1}\left(\tilde{x}_{k^{-} \mid  k^{-}}-\Psi F_{\kt}^{\top}\bar{Q}_{\kt}^{-1}\tilde{x}_{k\mid k^{-}}\right),
% \end{align*}
% which is quadratic in $\tilde{x}_{k \mid k^-}$. Subtracting $L_1\left(\tilde{x}_{k\mid k^{-}},\tilde{x}_{k^{-} \mid  k^{-}}\right)$ from $L$ gives the term
% \begin{equation}\label{eq:lgipdaf_uncertainty_L_tmp}
% L_2\left(\tilde{x}_{k\mid k^{-}}\right) =\frac{1}{2}\left(\tilde{x}_{k\mid k^{-}}^{\top}\left(\bar{Q}_{\kt}^{-1}-\bar{Q}_{\kt}^{-1}F_{\kt}\Psi F_{\kt}^{\top}\bar{Q}_{\kt}^{-1}\right)\tilde{x}_{k\mid k^{-}}\right),
% \end{equation}
% which is quadratic in $\tilde{x}_{k \mid k^-}$ and not dependent on $\tilde{x}_{k^- \mid k^-}$.
% Applying the inversion lemma presented in \cite{Thrun2006} to equation \eqref{eq:lgipdaf_uncertainty_L_tmp} and letting $P_{k \mid k^{-}} = \left(F_{\kt}P_{k \mid k^{-}}F_{\kt}^{\top}+\bar{Q}_{\kt}\right)$ gives 
% \[
% L_2\left(\tilde{x}_{k\mid k^{-}}\right)=\frac{1}{2}\tilde{x}_{k\mid k^{-}}^{\top}P^{-1}_{k\mid k^{-}}\tilde{x}_{k\mid k^{-}}.
% \]
\DIFdelbegin %DIFDELCMD < 

%DIFDELCMD < %%%
\DIFdelend %DIF >  
% Substituting in $L_1\left(\tilde{x}_{k\mid k^{-}},\tilde{x}_{k^{-} \mid  k^{-}}\right)$ and $L_2\left(\tilde{x}_{k\mid k^{-}}\right)$ for $L$ into equation~\eqref{eq:lgipdaf_prob_with_L} and pulling out $L_2\left(\tilde{x}_{k\mid k^{-}}\right)$ from the integral since it is not dependent on $\tilde{x}_{k^- \mid k^-}$ yields
\DIFaddbegin \DIFadd{and therefore
}\DIFaddend \begin{align*}
    p\left(x_{k}\mid \epsilon_{k^-}, Z_{0:k^-} \right) 
    % \\ \approx &\eta \exp{\left(- L_2\left(\tilde{x}_{k\mid k^{-}}\right)\right)} \\ &
    % \int_{\tilde{x}_{k^{-} \mid  k^{-}}}\exp\left(-L_1\left(\tilde{x}_{k\mid k^{-}},\tilde{x}_{k^{-} \mid  k^{-}}\right) \right)d \tilde{x}_{k^{-} \mid  k^{-}} \\
     =  \eta \exp{\left(- L_2\left(\xtkkm\right)\right)},
\end{align*}
where the integral of \DIFdelbegin \DIFdel{$\exp{-L_1}$ }\DIFdelend \DIFaddbegin \DIFadd{$\exp{\left(-L_1\right)}$ }\DIFaddend has been absorbed into the normalizing coefficient $\eta$.

Let 
\[
\Pkkm = F_\kt \Pkmkm F_\kt^\top + \bar{Q}_\kt
\]
and recall that $\tilde{x}_{k \mid k^{-}} = \LogI{\G{x}}{\hat{x}_{k\mid k^{-}}^{-1}  x_{k} }$, where \DIFdelbegin \DIFdel{, }\DIFdelend from Lemma~\ref{lem:lgipdaf_prob_prop_state} we have that $\hat{x}_{k\mid k^{-}}=f\left(\hat{x}_{k^{-} \mid  k^{-}},0,t_{\kt} \right)$.
Therefore, the Lemma follows by noting that $p\left(x_{k} \mid \epsilon_{k^-}, Z_{0:k^-} \right) \approx \mathcal{N}\left(\hat{x}_{k\mid k^{-}}, P_{k \mid k^{-}} \right)$.
%%%%%%%%%%%%%%%%%%%%%%%%%%%%%%%%%%%%%%%%%%%%%%%%
\end{proof}
