# Supplementary material for: The Integrated Probabilistic Data Association Filter Adapted to Lie Groups
Source: arXiv:2108.07265 source file (2022-10-14)
Supplement: Supplementary file 9 [file 06_LG_IPDAF.tex]

\section{Derivation of the LG-IPDAF\label{sec:lg_ipdaf}}

The integrated probabilistic data association filter incorporates all of the measurements inside a track's validation region in updating the track's state estimate,
error covariance and likelihood. The filter is derived using the pure minimum
mean square error (MMSE). We try to be as detailed as possible
in this derivation. 

Let 
\[
Z_{k}=\left\{ z_{k,j}\right\} _{j=1}^{m_{k}}
\]
denote the set of measurements in the track's validation region, $z_{k,j}$ denote the $j^{th}$ validated measurement, and $m_{k}$ denote the number of validated measurements at timestep $k$. The cumulative set of validated measurements from the initial time to timestep $k$ is denoted 
\[
Z_{0:k}=\left\{ Z_{\ell}\right\} _{\ell=0}^{k}.
\]

Let $\epsilon$ denote denote a Bernoulli random variable that represents the target's existence with
$
p\left(\top\epsilon_{k}\mid Z_{0:k}\right)
$
denoting the probability that the target the track represents exists conditioned on $Z_{0:k}$ and 
\[
p\left(\neg\epsilon_{k}\mid Z_{0:k}\right)=1-p\left(\top\epsilon_{k}\mid Z_{0:k}\right).
\]
denoting the probability that the target does not exist conditioned on $Z_{0:k}$. We refer to
$
p\left(\top\epsilon_{k}\mid Z_{0:k}\right)
$
as the track's likelihood. 
Lastly, let 
$
p\left(x_{k}\mid\top\epsilon_{k},Z_{0:k}\right)
$
denote the probability of a track's state conditioned on $\top\epsilon_{k}$ and $Z_{0:k}$. In the original derivation of the PDAF, it is assumed that the target exists; however, the IPDAF doesn't make that assumption so we must explicitly state this conditional dependency. When new measurements are received, the IPDAF uses them to update the track's likelihood and state probability. 

The IPDAF assumes that at most one measurement originates from
the target at every time step; thus, given the set of new measurements $Z_{k}$ either one of the measurements is target originated or none of them are. These possibilities are referred to as association events denoted $\theta_{k,j}$ with the subscript $j$ meaning that the $j^{th}$ measurement is target originated and all others are false, with $j=0$ meaning that all of the measurements are false. Hence, there are a total of $m_k+1$ association events. 

The probability of the track's state conditioned on the association event $\theta_{k,j}$ is
$
p\left(x_{k,j}\mid\theta_{k,j},\top\epsilon_{k},Z_{0:k}\right),
$
where $x_{k,j}$ is the state conditioned on $\theta_{k,j}$. This probability is derived in subsection \ref{subsec:Single-Event-Update} and referred to as the probability of the split track's state. The probability of the association event is
$
p\left(\theta_{k,j}\mid\top\epsilon_{k},Z_{0:k}\right),
$ and is derived in subsection \ref{subsec:association_event}. We will refer to this probability as $\beta_{k,j}$. Using the theorem of total probability to take into account all of the
association events, the track's state probability is 
\begin{equation}\label{eq:prob_state_cond_exist_meas}
p\left(x_{k}\mid\top\epsilon_{k},Z_{0:k}\right)  =\sum_{j=0}^{m_{k}}p\left(x_{k,j}\mid\theta_{k,j},\top\epsilon_{k},Z_{0:k}\right)\beta_{k,j}.
\end{equation}
In essence, the track's state probability is the weighted average of the split track's state probabilities. The process of splitting tracks would be repeated every time new measurements are received which would lead to an exponential growth of split tracks. This
process would quickly become very computationally and memory expensive. In order to keep it manageable, the split tracks can be fused together using the smoothing property of conditional expectations \cite{Bar-Shalom2001} adapted to Lie groups.
%
%
%%%%%%%%%%%%%%%%%%%%%%%%%%%%%%%%%%%%%%%%%%%%%%%%%%%%%%%%%%%%%%%%%%%%%%%%%%%%%%%%%%%
\subsection{State Estimation and Track's Likelihood Update}

Recall that the uncertainty for Lie groups is expressed in the Lie algebra using the error state as discussed in subsection \ref{ssec:uncertainty}. Thus, we can solve \eqref{eq:prob_state_cond_exist_meas} indirectly by solving 
\begin{equation}
 p\left(\tilde{x}_{k}\mid\top\epsilon_{k},Z_{0:k}\right)  =\sum_{j=0}^{m_{k}}p\left(\tilde{x}_{k,j}\mid\theta_{k,j},\top\epsilon_{k},Z_{0:k}\right)\beta_{k,j}.  
\end{equation}


Since the tangent space is an algebraic space, we can calculate the expected value of the track's error state using the smoothing property of conditional expectations. Let $\mu_{k,j} = \text{E}\left[\tilde{x}_{k,}\mid\top\epsilon_{k},Z_{0:k}\right]$ with $\mu_{k,0} = 0$ since the expected value of the error state is zero before updating, then  
\begin{subequations}\label{eq:expected_value}
\begin{align}
   \text{E}\left[ \tilde{x}_k\mid\top\epsilon_{k},Z_{0:k}\right] &=\text{E}\left[ \text{E}\left[ \tilde{x}_{k,j} | \theta_{k,j, \top\epsilon_{k},Z_{0:k}}\right]\right] \\
   & = \sum_{j=0}^{m_k} \text{E}\left[ \tilde{x}_{k,j} | \theta_{k,j, \top\epsilon_{k},Z_{0:k}}\right] \beta_{k,j}\\
   & = \sum_{j=0}^{m_k} \mu_{k,j} \beta_{k,j} \\
   & = \mu_k,
  \end{align}
\end{subequations}

where 
\begin{equation}\label{eq:prob_event_poisson}
\beta_{k,j}=\begin{cases}
\frac{\bar{p}\left(z_{k,j}\right)\frac{1}{\lambda}P_{D}}{\left(\frac{1}{\lambda}P_{D}\sum_{j=1}^{m_{k}}\bar{p}\left(z_{k,j}\right)+\left(1-P_{G}P_{D}\right)\right)} & j=1,\ldots,m_{k}\\
\frac{\left(1-P_{G}P_{D}\right)}{\left(\frac{1}{\lambda}P_{D}\sum_{j=1}^{m_{k}}\bar{p}\left(z_{k,j}\right)+\left(1-P_{G}P_{D}\right)\right)} & j=0,
\end{cases}
\end{equation}

and is derived in subsection \ref{subsec:association_event}.

In order to reset the expected value of $\tilde{x}_k$ to zero, $\mu_k$ is absorbed into the state estimate; thus, the state estimate update is
\begin{equation} \label{eq:state_estimate_update}
   \hat{x}_{k\mid k} = \hat{x}_{k\mid i}\oplus{\mu_k}.
\end{equation}

Using the updated expected value of the state estimate, the covariance is 
\begin{align*}
\text{cov}\left[x_{k}\mid\top\epsilon_{k},Z_{0:k}\right]= & \text{E}\left[\left(x_{k}\ominus\hat{x}_{k}\right)\left(x_{k}\ominus\hat{x}_{k}\right)^{\top}\mid\top\epsilon_{k},Z_{0:k}\right]\\
 & =\left(\sum_{i=0}^{m_{k}}\mu_{k,j}\beta_{k,j}\right)\left(\sum_{j=0}^{m_{k}}\mu_{k,j}\beta_{k,j}\right)^{\top}.
\end{align*}
From this point the derivation follows from \cite{Bar-Shalom2011} and results in
\[
P_{k\mid k}=\beta_{k,0}P_{k\mid i}+\left(1-\beta_{k,0}\right)P_{k\mid k}^{c}+\tilde{P}_{k\mid k}
\]
where 
%
\begin{align*}
\mu_{k,j} & = K_{k} \nu_{k,j}, \\
P_{k\mid k}^{c} & =P_{k\mid i}-K_{k} S_{k} K_{k}^{\top},\\
\tilde{P}_{k\mid k} & =K_{k}\left(\sum_{j=1}^{m_{k}}\beta_{k,j}\nu_{k,j}\nu_{k,j}^{\top}-\nu_{k}\nu_{k}^{\top}\right)K_{k}^{\top},
\end{align*}
%
$\nu_{k,j}$ is the innovation, $S_k$ is the innovation covariance and $K_k$ is the Kalman gain. The covariance term $P_{k\mid k}^c$ is the covariance updated from a single association event, and the covariance term $\tilde{P}_{k \mid k}$ captures the "spread of the means, $\tilde{x}_{k,j}"$. 

The terms $\nu_{k,j}$, $S_k$, and $K_k$ are derived from the update step of the indirect Kalman filter discussed in subsection \ref{subsec:Single-Event-Update}, and the derivation of  $\beta_{k,j}$ is given in subsection \ref{subsec:association_event}.

The track's likelihood is update is
%
\begin{equation} \label{eq:existence_final}
    p\left(\top\epsilon_{k}\mid Z_{0:k}\right) = \frac{1-\alpha_k}{1-\alpha_k  p\left(\top\epsilon_{k}\mid Z_{0:i}\right)}  p\left(\top\epsilon_{k}\mid Z_{0:i}\right),
\end{equation}
%
with 
%
\begin{equation}
    \alpha_{k} = 
    \begin{cases}
    P_D P_G & \text{if } m_k=0 \\
    P_D P_G - \frac{P_D}{\lambda}\sum_{j=1}^{m_{k}}\bar{p}\left(z_{k,j}\right) & \text{else},
    \end{cases},
\end{equation}
%
and  
\begin{subequations}
\begin{align*}
\bar{p}\left(z_{k,j}\right) & \triangleq p\left(z_{k,\ell}\mid \top \epsilon_{k},\theta_{k,j},m_{k},Z_{0:i}\right) \\
& = \mathcal{N}\left( z_{k,j} \ominus \hat{z}_{k,j}  , R_k\right).
\end{align*}
\end{subequations}
%
$\alpha_k$ is derived in subsection \ref{subsec:association_event}.






%%%%%%%%%%%%%%%%%%%%%%%%%%%%%%%%%%%%%%%%%%%%%%%%%%%%%%%%%%%%%%%%%%%%%%%%%%%%%%%%%

\subsection{Single Event Update\label{subsec:Single-Event-Update}}

In the single event update, we are interested in calculating $p\left(\tilde{x}_{k,j}\mid\theta_{k,j},\top\epsilon_{k},Z_{0:k}\right)$ using the measurement $z_{k,j}$, the prior probability, $p\left( \tilde{x}_k \mid \top\epsilon_{k}, Z_{0:i}\right)$, and the measurement probability conditioned on the target's state, association event, and the target's existence $\bar{p}\left(z_{k,j}\right)$. According to Bayes' rule 
%
\begin{equation}
    p\left(\tilde{x}_{k,j}\mid\theta_{k,j},\top\epsilon_{k},Z_{0:k}\right) = \frac{\bar{p}\left(z_{k,j}\right)p\left( \tilde{x}_k \mid\top\epsilon_{k}, Z_{0:i}\right)}{p\left(z_{k,j} \mid  \theta_{k,j} \right)}
\end{equation}

Using lemma \ref{lem:posterior}, the maximum a posteriori (MAP) solution is 
%
\begin{align*}
    & p\left(\tilde{x}_{k,j}\mid\theta_{k,j},\top\epsilon_{k},Z_{0:k}\right)= \\
    &\eta\exp\left(\left(\tilde{x}_{k|k} - \mu_{k|k}\right)^{\top}P_{k|k}^{-1}\left(\tilde{x}_{k|k} - \mu_{k|k}\right)\right),
\end{align*}
where 
\begin{align*}
\hat{z}_{k,j} & =h\left(x_{k|i},0\right)\\
\nu_{k,j} & =z_{k,j}\ominus\hat{z}_{k}\\
S_{k} & =H_{k}P_{k|i}H_{k}^{\top}+V_{k}R_{k}V_{k}^{\top}\\
K_{k} & =P_{k|i}H_{k}^{\top}S_{k}^{-1}\\
\mu_{k,j} & =K_{k}\nu_{k,j}\\
P_{k|k,j} & = \left(I-K_{k} H_{k}\right)P_{k|i},
\end{align*}
and the Jacobians $H_{k}$ and $V_{k}$ are defined in \eqref{eq:system_jacobians}. Note that we have not reset the mean of $\tilde{x}_{k|k}$ to zero by absorbing the mean $\mu_{k,j}$ into the state estimate $\hat{x}_{k|i}$ as done in lemma \ref{lem:posterior}. This is because we need the means to be in the same tangent space in order to fuse them together. After fusing them, the fused mean is moved to the state estimate $\hat{x}_{k|i}$ as stated in equations \eqref{eq:expected_value} and \eqref{eq:state_estimate_update}.




%%%%%%%%%%%%%%%%%%%%%%%%%%%%%%%%%%%%%%%%%%%%%%%%%%%%%%%%%%%%%%%%%%%%%%%%%%%%%%%%%%

\subsection{Data Association}\label{subsec:association_event}

We can infer the probability of an association event
and the track's likelihood using the location of the measurements and the number of measurements
at each time step. The basic idea is that under the assumption that
the expected number of false measurements are uniformly distributed
in the surveillance region, we would expect a certain number of false
measurements in the validation region of the target. If the number
of measurements in the validation region is less than or equal to
the expected number of false measurements, then it is more likely
that all of the measurements are false and that the target does not
exist; similarly, if the number of measurements in the validation
region is greater than the expected number of false measurements,
then it is more likely that one of the measurements is target originated
and the target exists. Also, the closer a measurement is to the state
estimate of a track the more probable the association event
is and the more probable the target exists. We explicitly write this
inference using a discrete joint distribution as 
%
\begin{equation}
p\left(\epsilon_{k},\theta_{k,j}\mid Z_{0:k}\right)=p\left(\epsilon_{k},\theta_{k,j}\mid Z_{k},m_{k},Z_{0:i}\right).\label{eq:discrete_joint_existance_event}
\end{equation}
%
where we have separated $Z_k$ from $Z_{k:i}$ since the new measurements will be used to update the joint distribution. 


% from which we can compute the marginal distributions
% \begin{subequations} \label{eq:marginal_distributions}
% \begin{align}
% p\left(\theta_{k,j}\mid Z_{0:k}\right) & =p\left(\top\epsilon_{k},\theta_{k,j}\mid Z_{0:k}\right)+p\left(\neg\epsilon_{k},\theta_{k,j}\mid Z_{0:k}\right)\label{eq:marginal_event}\\
% p\left(\top\epsilon_{k}\mid Z_{0:k}\right) & =p\left(\top\epsilon_{k},\theta_{k,0}\mid Z_{0:k}\right)+\sum_{j=1}^{m_{k}}p\left(\top\epsilon_{k},\theta_{k,j}\mid Z_{0:k}\right)\label{eq:marginal_exists}\\
% p\left(\neg\epsilon_{k}\mid Z_{0:k}\right) & =p\left(\neg\epsilon_{k},\theta_{k,0}\mid Z_{0:k}\right)\label{eq:marginal_doesnt_exist}
% \end{align}
% \end{subequations}
% noting that 
% \[
% p\left(\neg\epsilon_{k},\theta_{k,j}\mid Z_{0:k}\right)=0\quad\text{for }j=1,\ldots,m_{k},
% \]
% since if the target doesn't exist, then none of the measurements can
% be target oriented. 

Using Bayes' rule, the joint distribution in equation \eqref{eq:discrete_joint_existance_event} is 

\begin{align}\label{eq:liklihood_event_join_distribution}
p\left(\epsilon_{k},\theta_{k,j}\mid Z_{0:k}\right) & =  \frac{1}{c} p\left(Z_{k}\mid\epsilon_{k},\theta_{k,j},m_{k},Z_{0:i}\right) \notag \\ &  p\left(\epsilon_{k},\theta_{k,j}\mid m_{k},Z_{0:i}\right), \\
c & = \sum_{j=0}^{m_{k}}\left(p\left(Z_{k}\mid\epsilon_{k},\theta_{k,j},m_{k},Z_{0:i}\right)\right. \notag \\ &\left. p\left(\epsilon_{k},\theta_{k,j}\mid m_{k},Z_{0:i}\right)\right). \label{eq:coefficient_c}
\end{align}

%%%%%%%%%%%%%%%%%%%%%%%%%%%%%%%%%%%%%%%%%%%%%%%%%%%%%%%
Assuming that the measurements in the validation region are independent, the joint distribution of the measurements is the product of the distribution of each measurement;
\begin{equation}\label{eq:meas_prod}
p\left(Z_{k}\mid\epsilon_{k},\theta_{k,j},m_{k},Z_{0:i}\right)=\prod_{\ell=1}^{m_{k}}p\left(z_{k,\ell}\mid\epsilon_{k},\theta_{k,j},m_{k},Z_{0:i}\right).
\end{equation}

Recalling that the false measurements are uniformly
distributed in the validation region with volume $\mathcal{V}_k$ and gate probability $P_G$, the probability of each measurement is
%
% \begin{subequations}
\begin{align}
& p\left(z_{k,\ell}\mid\epsilon_{k},\theta_{k,j},m_{k},Z_{0:i}\right) \notag \\
& = \begin{cases}
\mathcal{V}_{k}^{-1} & \text{if }j\neq \ell\text{ and } \epsilon_k =\top \epsilon_k \\
0 & \text{if }j\neq 0 \text{ and } \epsilon_k =\neg \epsilon_k \\
P_{G}^{-1}\bar{p}\left(z_{k,\ell}\right) & \text{if }j = \ell\text{ and } \epsilon_k =\top \epsilon_k
\end{cases}\label{eq:meas_prob_cond}  ,
\end{align}
% \end{subequations}
%
where $P_{G}^{-1}\bar{p}\left(z_{k,\ell}\right)$ is the probability of the measurement conditioned on it being in the validation region. 

Using equations \eqref{eq:meas_prod} and \eqref{eq:meas_prob_cond}, the joint distribution of the measurements is
%
\begin{align} \label{eq:joint_dist_meas}
& p\left(Z_{k}\mid\epsilon_{k},\theta_{k,j},m_{k},Z_{0:i}\right) \notag \\ 
&=\begin{cases}
\mathcal{V}_{k}^{-m_{k}+1}P_{G}^{-1}\bar{p}\left(z_{k,j}\right) & j \in \mathbb{M}\text{ and }\epsilon_{k}=\top\epsilon_{k}\\
\mathcal{V}_{k}^{-m_{k}} & j=0\\
0 & j=\in \mathbb{M} \text{ and }\epsilon_{k}=\neg\epsilon_{k}
\end{cases},
\end{align}
%
where $\mathbb{M}=\left\{1,\ldots,m_k\right\}$.

The joint distribution of the target's existence and the association event is 
\begin{align} \label{eq:joint_dist_existence_event_final_a}
& p\left(\epsilon_{k},\theta_{k,j}\mid m_{k},Z_{0:i}\right) \notag \\
  & =\begin{cases}
\frac{1}{\gamma m_{k}}P_{D}P_{G}P_{T}\mu_{F}\left(m_{k}-1\right) & j \in \mathbb{M}\text{ and }\top\epsilon_{k}\\
\frac{1}{\gamma}\left(1-P_{G}P_{D}\right)P_{T}\mu_{F}\left(m_{k}\right) & j=0\text{ and }\top\epsilon_{k}\\
0 & j \in \mathbb{M}\text{ and }\neg\epsilon_{k}\\
\frac{1}{\gamma}\left(1-P_{T}\right)\mu_{F}\left(m_{k}\right) & j=0\text{ and }\neg\epsilon_{k}
\end{cases},
\end{align}
%
with 
$$
\gamma = P_{G}P_{D}P_{T}\mu_{F}\left(m_{k}-1\right)+\left(1-P_{G}P_{D}P_{T}\right)\mu_{F}\left(m_{k}\right).
$$
%
The above joint distirbution is derived in subsection \ref{subsec:track_likelihood_and_event_joint}. 

Substituting equations \eqref{eq:joint_dist_meas} and \eqref{eq:joint_dist_existence_event_final_a} into \eqref{eq:liklihood_event_join_distribution} yields
%
%
% \begin{align*}
% c =\frac{\mathcal{V}_{k}^{^{-m_{k}}}\left[\left(1-P_{G}P_{D}P_{T}\right)\mu_{F}\left(m_{k}\right)+\frac{1}{m_{k}}P_{D}P_{T}\mathcal{V}_{k}\mu_{F}\left(m_{k}-1\right)\sum_{i=1}^{m_{k}}\bar{p}\left(z_{i}\right)\right]}{P_{G}P_{D}P_{T}\mu_{F}\left(m_{k}-1\right)+\left(1-P_{G}P_{D}P_{T}\right)\mu_{F}\left(m_{k}\right)}.
% \end{align*}
% 
% 
\begin{align} \label{eq:joint_prob_existence_event_final}
& p\left(\epsilon_{k},\theta_{k,j}\mid Z_{0:k}\right) \notag \\
& =\begin{cases}
\frac{1}{\xi m_{k}}\mathcal{V}_{k}\bar{p}\left(z_{k,i}\right)P_{D}P_{T}\mu_{F}\left(m_{k}-1\right) & j \in \mathbb{M}\text{ and }\top\epsilon_{k}\\
\frac{1}{\xi} \left(1-P_{G}P_{D}\right)P_{T}\mu_{F}\left(m_{k}\right) & j=0\text{ and }\top\epsilon_{k}\\
0 & j \in \mathbb{M}\text{ and }\neg\epsilon_{k}\\
\frac{1}{\xi} \left(1-P_{T}\right)\mu_{F}\left(m_{k}\right) & j=0\text{ and }\neg\epsilon_{k}.
\end{cases}
\end{align}
%
with 
\begin{align*}
\xi &= \left(1-P_{G}P_{D}P_{T}\right)\mu_{F}\left(m_{k}\right) \\& +\frac{1}{m_{k}}P_{D}P_{T}\mathcal{V}_{k}\mu_{F}\left(m_{k}-1\right)\sum_{j=1}^{m_{k}}\bar{p}\left(z_{j}\right)
\end{align*}
%
We can compute the marginal distributions of equation \eqref{eq:joint_prob_existence_event_final} to calculate $p\left(\top\epsilon_{k}\mid Z_{0:k}\right)$ and  $\beta_{k,j}$. 
%
\begin{subequations}\label{eq:existence_general}
\begin{align*}
&p\left(\top\epsilon_{k}\mid Z_{0:k}\right) =\sum_{j=0}^{m_{k}}p\left(\top\epsilon_{k},\theta_{k,j}\mid Z_{0:k}\right)\\
 & =\frac{1}{\xi m_k}[\mathcal{V}_{k}P_{D}\mu_{F}\left(m_{k}-1\right)\sum_{j=1}^{m_{k}}\bar{p}\left(z_{k,j}\right)\\
 & \left.+m_k\left(1-P_{G}P_{D}\right)\mu_{F}\left(m_{k}\right)\right]P_{T},
\end{align*}
\end{subequations}
%
and $\beta_{k,j}$ is
%
\begin{equation}\label{eq:prob_event_general}
 \beta_{k,j}
 =\begin{cases}
\frac{1}{\zeta m_{k}}\mathcal{V}_{k}\bar{p}\left(z_{k,i}\right)P_{D}\mu_{F}\left(m_{k}-1\right) & j \in \mathbb{M}\\
\frac{1}{\zeta}\left(1-P_{G}P_{D}\right)\mu_{F}\left(m_{k}\right) & j=0
\end{cases},
\end{equation}

with
\begin{align*}
    \zeta & = \mathcal{V}_{k}\frac{1}{m_{k}}P_{D}\mu_{F}\left(m_{k}-1\right)\sum_{j=1}^{m_{k}}\bar{p}\left(z_{k,j}\right) \\
    &+\left(1-P_{G}P_{D}\right)\mu_{F}\left(m_{k}\right).
\end{align*}

The probability distribution of the number of false measurements in the validation region is often modeled using a Poisson distribution defined as 
\begin{equation}
    \mu_{F}\left(m_{k}\right)=\exp\left(-\lambda \mathcal{V}_k\right)\frac{\left(\lambda \mathcal{V}_k\right)^{m_{k}}}{m_{k}!}
\end{equation}

where $\lambda$ is the spacial density of false measurements. Substituting in the Poisson distribution to equations \eqref{eq:existence_general} and \eqref{eq:prob_event_general} yields the equations \eqref{eq:existence_final} and \eqref{eq:prob_event_poisson}.



%%%%%%%%%%%%%%%%%%%%%%%%%%%%%%%%%%%%%%%%%%%%%%%%%%%%%%%%%%
\subsection{Target's Existence and Association Event Joint Distribution} \label{subsec:track_likelihood_and_event_joint}

In this subsection we derive the joint distribution of the target's existence and the association event defined in equation \eqref{eq:liklihood_event_join_distribution}. This derivation will be broken down into smaller steps by deriving the probabilities $p\left(\theta_{k,j}\mid\top\epsilon_{k},m_{k},Z_{0:i}\right)$, $p\left(\theta_{k,j}\mid\neg\epsilon_{k},m_{k},Z_{0:i}\right)$, $p\left(\top\epsilon_{k}\mid m_k,Z_{0:i}\right)$ and $p\left(\neg\epsilon\mid m_k,Z_{0:i}\right)$, and then using these probabilities with the theorem of total probability to get
%
\begin{align} \label{eq:joint_dist_existence_event}
    & p\left(\epsilon_{k},\theta_{k,j}\mid m_{k},Z_{0:i}\right) \notag \\  &=p\left(\theta_{k,j}\mid\top\epsilon_{k},m_{k}\right)p\left(\top\epsilon_{k}\mid m_{k}, Z_{0:i}\right) \notag \\
    &+p\left(\theta_{k,j}\mid\neg\epsilon_{k},m_{k}\right)p\left(\neg\epsilon_{k}\mid m_{k}, Z_{0:i}\right).
\end{align}

In the calculations that follow, let $\phi$ denote the number of
false measurements. Under the assumption that there is
at most one target oriented measurement, there are two possibilities
for the number of false measurements, $\phi = {m_k}$, denoted $\phi_{m_k}$, or $\phi = {m_k -1}$ denoted $\phi_{m_k^-}$. Therefore, the a priori probability of an event conditioned on the
number of measurements, the target's existence, and previous measurements is 
%
\begin{align}\label{eq:event_cond_prob}
& p\left(\theta_{k,j}\mid\top\epsilon_{k},m_{k},Z_{0:i}\right) \notag \\
&=p\left(\theta_{k,j}\mid\top\epsilon_{k},\phi_{m_k^-},m_{k},Z_{0:i}\right)p\left(\phi_{m_k^-}\mid\top\epsilon_{k},m_{k},Z_{0:i}\right)\notag\\
 & +p\left(\theta_{k,j}\mid\top\epsilon_{k},\phi_{m_k},m_{k},Z_{0:i}\right)p\left(\phi_{m_k}\mid\top\epsilon_{k},m_{k},Z_{0:i}\right)\notag\\
 & =\begin{cases}
\left(\frac{1}{m_{k}}\right)p\left(\phi_{m_k^-}\mid\top\epsilon_{k},m_{k},Z_{0:i}\right) & j=1,\ldots,m_{k}\\
p\left(\phi_{m_k}\mid\top\epsilon_{k},m_{k},Z_{0:i}\right) & i=0.
\end{cases}
\end{align}

Using Bayes' formula, the conditional probabilities of the number of false measurements are
%
\begin{align}\label{eq:num_false_meas_cond_prob}
& p\left(\phi_{m_k^-}\mid\top\epsilon_{k},m_{k},Z_{0:i}\right) \notag \\
&=\frac{p\left(m_{k}\mid\phi_{m_k^-},\top\epsilon_{k},Z_{0:i}\right)p\left(\phi_{m_k^-}\mid\top\epsilon_{k},Z_{0:i}\right)}{p\left(m_{k}\mid\top\epsilon_{k},Z_{0:i}\right)}\notag\\
 & =\frac{P_{G}P_{D}\mu_{F}\left(m_{k}-1\right)}{p\left(m_{k}\mid\top\epsilon_{k},Z_{0:i}\right)}\\
& p\left(\phi_{m_k}\mid\top\epsilon_{k},m_{k},Z_{0:i}\right) \notag \\
&=\frac{p\left(m_{k}\mid\phi_{m_k},\epsilon_{k},Z_{0:i}\right)p\left(\phi_{m_k}\mid\top\epsilon_{k},Z_{0:i}\right)}{p\left(m_{k}\mid\top\epsilon_{k},Z_{0:i}\right)}\notag\\
 & =\frac{\left(1-P_{G}P_{D}\right)\mu_{F}\left(m_{k}\right)}{p\left(m_{k}\mid\top\epsilon_{k},Z_{0:i}\right)}.
\end{align}
%
where $\mu_{F}$ is the probability density function of the number
of false measurements.
Using the theorem of total probability
%
\begin{align}\label{eq:num_meas_prob}
& p\left(m_{k}\mid\top\epsilon_{k},Z_{0:i}\right) \notag \\
&=p\left(m_{k}\mid\phi_{m_k^-},\top\epsilon_{k},Z_{0:i}\right)p\left(\phi_{m_k^-}\mid\top\epsilon_{k},Z_{0:i}\right) \notag\\
&+p\left(m_{k}\mid\phi_{m_k},\top\epsilon_{k},Z_{0:i}\right)p\left(\phi_{m_k}\mid\top\epsilon_{k},Z_{0:i}\right)\notag\\
 & =\chi,
\end{align}
where
\begin{equation}
    \chi = P_{G}P_{D}\mu_{F}\left(m_{k}-1\right)+\left(1-P_{G}P_{D}\right)\mu_{F}\left(m_{k}\right).
\end{equation}

Combining equations \eqref{eq:event_cond_prob}, \eqref{eq:num_false_meas_cond_prob}, and \eqref{eq:num_meas_prob} yields
\begin{align}\label{eq:event_cond_prob_exist_final}
&p\left(\theta_{k,j}\mid\top\epsilon_{k},m_{k},Z_{0:i}\right) \notag \\
&=\begin{cases}
\frac{\frac{1}{m_{k}}P_{D}P_{G}\mu_{F}\left(m_{k}-1\right)}{P_{G}P_{D}\mu_{F}\left(m_{k}-1\right)+\left(1-P_{G}P_{D}\right)\mu_{F}\left(m_{k}\right)} & j\in \mathbb{M}\\
\frac{\left(1-P_{G}P_{D}\right)\mu_{F}\left(m_{k}\right)}{P_{G}P_{D}\mu_{F}\left(m_{k}-1\right)+\left(1-P_{G}P_{D}\right)\mu_{F}\left(m_{k}\right)} & j=0
\end{cases}.
\end{align}

The a priori probability of an event conditioned on the number of
measurements, previous measurements, and that the target does not exist is
\begin{equation}\label{eq:event_cond_prob_noexist_final}
p\left(\theta_{k,j}\mid\neg\epsilon_{k},m_{k},Z_{0:i}\right) =\begin{cases}
0 & j=1,\ldots,m_{k}\\
1 & j=0
\end{cases}.
\end{equation}

%%%%%%%

Next we calculate the probabilities $p\left(\top\epsilon_{k}\mid m_k,Z_{0:i}\right)$
and $p\left(\neg\epsilon\mid m_k,Z_{0:i}\right)$.
\begin{align*}
&p\left(\top\epsilon_{k}\mid m_{k},Z_{0:i}\right) \\
&=\frac{p\left(m_{k}\mid\top\epsilon_{k},Z_{0:i}\right)p\left(\top\epsilon_{k} \mid Z_{0:i}\right)}{p\left(m_{k}\mid Z_{0:i}\right)}\\
 & =\frac{\left(P_{G}P_{D}\mu_{F}\left(m_{k}-1\right)+\left(1-P_{G}P_{D}\right)\mu_{F}\left(m_{k}\right)\right)P_{T}}{p\left(m_{k}\mid Z_{0:i}\right)} \\
&p\left(\neg\epsilon\mid m_{k},Z_{0:i}\right) \\
& =\frac{p\left(m_{k}\mid\neg\epsilon_{k} \mid Z_{0:i}\right)p\left(\neg\epsilon_{k},Z_{0:i}\right)}{p\left(m_{k}\mid Z_{0:i}\right)}\\
 & =\frac{\mu_{F}\left(m_{k}\right)\left(1-P_{T}\right)}{p\left(m_{k}\mid Z_{0:i}\right)},
\end{align*}
where $P_{T}=p\left(\top\epsilon_{k},Z_{0:i}\right)$, and $p\left(m_{k}\mid Z_{0:i}\right)= \gamma$.

Therefore,
\begin{subequations}\label{eq:prob_existence_cond}
\begin{align}
p\left(\top\epsilon_{k}\mid m_{k},Z_{0:i}\right) &=\frac{\chi}{\gamma} P_{T}\\
p\left(\neg\epsilon\mid m_{k},Z_{0:i}\right) & =\frac{1}{\gamma}\mu_{F}\left(m_{k}\right)\left(1-P_{T}\right).
\end{align}
\end{subequations}

Using equations \eqref{eq:joint_dist_existence_event}, \eqref{eq:event_cond_prob_exist_final}, \eqref{eq:event_cond_prob_noexist_final}, and \eqref{eq:prob_existence_cond} the probability $p\left(\epsilon_{k},\theta_{k,j}\mid m_{k},Z_{0:i}\right)$ is \eqref{eq:joint_dist_existence_event_final_a}.


%%%%%%%%%%%%%%% solve for c %%%%%%%%%%%%%%%



% \begin{equation} \label{eq:joint_prob_existence_event_final}
% p\left(\epsilon_{k},\theta_{k,j}\mid Z_{0:k}\right) 
% =\begin{cases}
% \frac{1}{c}\frac{\mathcal{V}_{k}^{-(m_{k}+1)}\bar{p}\left(z_{k,i}\right)\frac{1}{m_{k}}P_{D}P_{T}\mu_{F}\left(m_{k}-1\right)}{P_{G}P_{D}P_{T}\mu_{F}\left(m_{k}-1\right)+\left(1-P_{G}P_{D}P_{T}\right)\mu_{F}\left(m_{k}\right)} & i=1,\ldots,m_{k}\text{ and }\top\epsilon_{k}\\
% \frac{1}{c}\frac{\mathcal{V}_{k}^{-m_{k}}\left(1-P_{G}P_{D}\right)P_{T}\mu_{F}\left(m_{k}\right)}{P_{G}P_{D}P_{T}\mu_{F}\left(m_{k}-1\right)+\left(1-P_{G}P_{D}P_{T}\right)\mu_{F}\left(m_{k}\right)} & i=0\text{ and }\top\epsilon_{k}\\
% 0 & i=1,\ldots,m_{k}\text{ and }\neg\epsilon_{k}\\
% \frac{1}{c}\frac{\mathcal{V}_{k}^{-m_{k}}\left(1-P_{T}\right)\mu_{F}\left(m_{k}\right)}{P_{G}P_{D}P_{T}\mu_{F}\left(m_{k}-1\right)+\left(1-P_{G}P_{D}P_{T}\right)\mu_{F}\left(m_{k}\right)} & i=0\text{ and }\neg\epsilon_{k}
% \end{cases}
% \end{equation}
