# Supplementary material for: The Integrated Probabilistic Data Association Filter Adapted to Lie Groups
Source: arXiv:2108.07265 source file (2022-10-14)
Supplement: Supplementary file 10 [file A1_DerivationOfJacobians.tex]

\section{Derivation of Jacobians\label{sec:DerivationOfJacobians}}

This appendix presents the derivation of the system Jacobians defined in \eqref{eq:system_jacobians}. The derivation follows the procedure described in \cite{Sola2018}. To simplify notation we will drop the subscripts denoting time where not needed. Note that we will take derivatives with respect to vectors in order to compress the derivation; however, keep in mind that the derivatives are being taken w.r.t. one component of at a time. 



\begin{lem}
\label{lem:transition_func_jacobians} Let the system model be defined as in \eqref{eq:system_model}, then the system Jacobians in matrix notation are defined in \eqref{eq:system_jacobians}.
\end{lem}





\begin{IEEEproof}
We begin by deriving the Jacobian $F$. By definition
%
\begin{align*}
F & =\lim_{\tilde{x}\to0}\frac{f\left(x\oplus\tilde{x}\right)\ominus f\left(x\right)}{\tilde{x}}\\
 & =\lim_{\tilde{x}\to0}\frac{1}{\tilde{x}}\text{Log}\left(g\text{Exp}\left(\tilde{g}\right)\text{Exp}\left(U+\delta_{i:k}\tilde{v}\right),\right.\\
 & \left.v +q^{v}+\tilde{v}\right)\ominus\left(g\text{Exp}\left(U\right),v+ w^{v}\right)\\
 & =\lim_{\tilde{x}\to0}\frac{\text{Log}\left(\text{Exp}\left(-U\right)\text{Exp}\left(\tilde{g}\right)\text{Exp\ensuremath{\left(U+\delta_{i:k}\tilde{v}\right)}},\tilde{v}\right)}{\tilde{x}}\\
 & =\lim_{\tilde{x}\to0}\frac{1}{\tilde{x}}\text{Log}\left(\text{Exp}\left(\mathbf{Ad}_{\text{Exp}\left(-U\right)}\tilde{g}\right)\text{Exp}\left(-U\right)\right.\\
 & \left.\text{Exp\ensuremath{\left(U+\delta_{i:k}\tilde{v}\right)}},\tilde{v}\right).
\end{align*}
%
The term can be simplified using the Baker Campbell Hausdorff (BCH)
formula and removing all second order and higher terms of $\tilde{x}$
since they will go to zero. This yields
%
\begin{align*}
F & =\lim_{\tilde{x}\to0}\frac{\left(\mathbf{Ad}_{\text{Exp}\left(-U\right)}\tilde{g}+\delta_{i:k} J_{r}\left(U\right)\tilde{v},\tilde{v}\right)}{\tilde{x}}. 
\end{align*}
%
Using matrix notation, we finally get 
%
\begin{align*}
F & =\lim_{\tilde{x}\to0}\begin{bmatrix}\mathbf{Ad}_{\text{Exp}\left(-U\right)} & J_{r}\left(U\right)\\
0_{n\times n} & I_{n\times n}
\end{bmatrix}\frac{\tilde{x}}{\tilde{x}}\\
 & =\begin{bmatrix}\mathbf{Ad}_{\text{Exp}\left(-U\right)} & J_{r}\left(U\right)\\
0_{n\times n} & I_{n\times n}
\end{bmatrix}.
\end{align*}
%
Next we derive the Jacobian $G$. By definition
%
\begin{align*}
G & =\lim_{\tilde{q}\to0}\frac{1}{\tilde{q}}\left(g\text{Exp}\left(U+\tilde{q}^{g}+\delta_{i:k}\tilde{q}^{v}\right),\right.\\
 & \left.u+ q^{v}+\tilde{q}^{v}\right)\ominus\left(g\text{Exp}\left(U\right),v+ q^{v}\right)\\
 & =\lim_{\tilde{q}\to0}\frac{\text{Log}}{\tilde{q}}\left(\text{Exp}\left(-U\right)\text{Exp}\left(U+\tilde{q}^{g}+\delta_{i:k}\tilde{q}^{v}\right),\right.\\
 & \left.\tilde{q}^{v}\right).
\end{align*}
Once again, the term can be simplified using the BCH formula by removing
all second order and higher terms of $\tilde{q}$ since they will go
to zero. This step yields
\[
G=\lim_{\tilde{q}\to0}\frac{\left( J_{r}\left(U\right)\tilde{q}^{g}+\delta_{i:k} J_{r}\left(U\right)\tilde{q}^{v},\tilde{q}^{v}\right)}{\tilde{q}}.
\]
Using matrix notation, we finally get 
\begin{align*}
G & =\lim_{\tilde{q}\to0}\begin{bmatrix} J_{r}\left(U\right) & \delta_{i:k} J_{r}\left(U\right)\\
0_{n\times n} &  I_{n\times n}
\end{bmatrix}\frac{\tilde{q}}{\tilde{q}}\\
 & =\begin{bmatrix} J_{r}\left(U\right) & \delta_{i:k} J_{r}\left(U\right)\\
0_{n\times n} & I_{n\times n}
\end{bmatrix}.
\end{align*}

The derivation of the observation function Jacobians are trivial and will not be shown here. 
\end{IEEEproof}
