# Supplementary material for: The Integrated Probabilistic Data Association Filter Adapted to Lie Groups
Source: arXiv:2108.07265 source file (2022-10-14)
Supplement: Supplementary file 11 [file A2_UncertaintyCalculations.tex]

%\section{Uncertainty Calculations\label{sec:uncertainty_calculations}}
